# Supplementary material for: Investigating Ground-level Ozone Formation: A Case Study in Taiwan
Source: arXiv:2012.10058 source file (2021-05-05)
Supplement: Supplementary file 1 [file 5_Appendix.tex]

\setcounter{figure}{0} 
\setcounter{table}{0} 

\section{Supplementary: Appendix}
\subsection{Dataset}

\iffalse 
\subsection{Definition of model performance evaluation terms}
Slope, RMSE, and $\textrm R^{2}$ are used to evaluate the performance of models. \\
The slope is computed as follows:
 \[slope = 1-\frac{\sum_{i=1}^{m}(O_{3_{\:(obs)}\:i}O_{3_{\:(pred)}\:i}-O_{3_{\:(obs)}\:i}\overline{O_3}_{\:(pred)})}{\sum_{i=1}^{m}((O_{3_{\:(obs)}\:i})^2-O_{3_{\:(obs)}\:i}\overline{O_3}_{\:(obs)})}\]
The RMSE is computed as follows:
\[RMSE = \sqrt{\frac{1}{m}\sum_{i=1}^{m}(O_{3_{\:(pred)}\:i}-O_{3_{\:(obs)}\:i})^2}\]

The $\textrm R^{2}$ is computed as follows:
 \[R^2 = 1-\frac{\sum_{i=1}^{m}(O_{3_{\:(pred)}\:i}-O_{3_{\:(obs)}\:i})^2}{\sum_{i=1}^{m}(\overline{O_3}_{\:(obs)}-O_{3_{\:(obs)}\:i})^2}\]

where $\overline{O_3}_{\:(obs)}$ and $\overline{O_3}_{\:(pred)}$ are the average of observed \ce{O3} and model-predicted \ce{O3}, respectively.
%\clearpage

\subsection{Additional results}
\label{sec:additional_results}
The 10-fold cross-validation is applied on the training of each model to verify the stability of optimized models. Three division ways are conducted to decide validation data for the 10-fold validation, including 10\% randomized sample, 10\% randomized stations, and 10\% of dates. Table \ref{tab:model_performance} and Figure \ref{fig:index_pred2obs} show the results.
\fi
